# Supplementary material for: Pressure-Induced Volume Collapse and Metallization in Inverse Spinel Co$_2$TiO$_4$
Source: arXiv:2504.00574 ancillary file (2025-06-28)
Supplement: Supplementary file 1 [file Supplementary__Pressure_Induced_Volume_Collapse_and_Metallization_in_Inverse_Spinel_Co_2TiO_4.pdf]

# Supplementary: Pressure-Induced Volume Collapse and Metallization in Inverse Spinel $Co_2TiO_4$

Mrinmay Sahu,[1,2] Souvick Chakraborty,[1] Bidisha Mukherjee,[1,2] Bishnupada Ghosh,[1,2,3]
Asish Kumar Mishra,[1,2] Satyabrata Raj,[1,2] and Goutam Dev Mukherjee[1,2,*]

[1]*Department of Physical Sciences, Indian Institute of Science Education and Research Kolkata, Mohanpur, Nadia, West Bengal-741246, India*

[2]*National Centre for High Pressure Studies, Indian Institute of Science Education and Research Kolkata, Mohanpur, Nadia, West Bengal-741246, India*

[3]*Diamond Light Source Ltd, Harwell Science and Innovation Campus, Didcot OX11 0DE, United Kingdom*

[*] Corresponding Author:goutamdev@iiserkol.ac.in

## S1 Field Emission Scanning Electron Microscopy (FESEM) images

The morphologies of the inverse spinel $Co_2TiO_4$ (CTO-Sp) powder sample were examined by SUPRA 55 VP-4132 CARL ZEISS FESEM running at 5.21 KeV. Figure 1(a) shows the scanning electron microscopy (SEM) images of prepared polycrystalline $Co_2TiO_4$ powder. To measure the particle size we have used the ImageJ software. The particle size distribution is shown in Figure 1(b). From the particle size distribution graph, the average particle size is estimated to 2.75 $\mu$m which is comparable with others [1, 2].

## S2 Energy Dispersive X-ray Spectroscopy (EDX)

Elemental components were accomplished by employing energy-dispersive x-ray (EDX,........) of the $Co_2TiO_4$ sample. We have taken the EDX data for the three different positions of the sample surface as indicated in the Figure 2(a),(b)and (c). Along with the elemental mapping of CTO-Sp, atomic percentages are also mentioned in the figure. Accurately determining the atomic percentage of oxygen using EDX has its challenges and limitations.

---


[1] Q. S. Fu, C. L. Li, B. Meng, C. Chakrabarti, R. Zhang, X. H. Chen, Y. H. Li, S. L. Yuan, Ceram. Int. **45**, 6906 (2019).

[2] S. Nayak, K. Dasari, D. C. Joshi, P. Pramanik, R. Palai, V. Sathe, R. N. Chauhan, N. Tiwari, and S. Thota, Phys. Status Solidi B **253**, 2270 (2016).

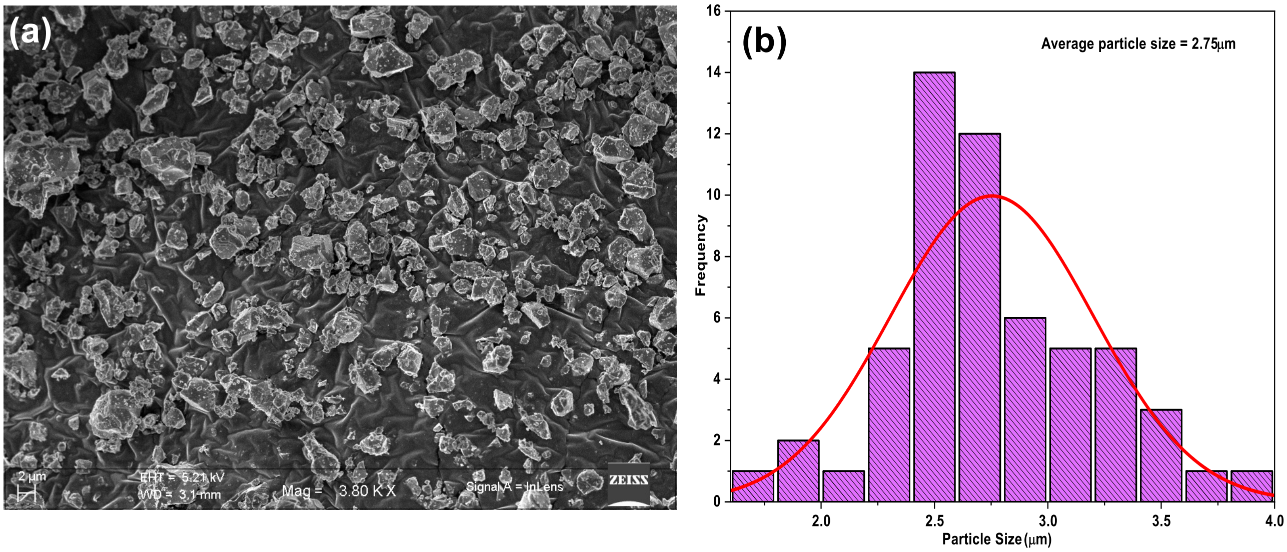


Figure S1. (a) Scanning Electron Microscopy (SEM) images of powder CTO-Sp. (b) Particle size distribution of polycrystalline CTO-Sp.

**Position 1**

| Elem... | Weight% | Atomic% |
|---|---|---|
| O K | 36.60 | 66.61 |
| Ti K | 18.17 | 11.04 |
| Co K | 45.23 | 22.35 |
| Totals | 100.00 | |

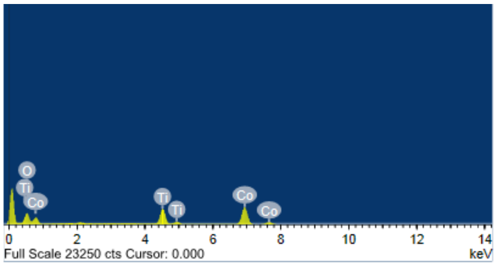


**Position 2**

| Elem... | Weight% | Atomic% |
|---|---|---|
| O K | 37.27 | 67.25 |
| Ti K | 17.89 | 10.78 |
| Co K | 44.83 | 21.96 |
| Totals | 100.00 | |

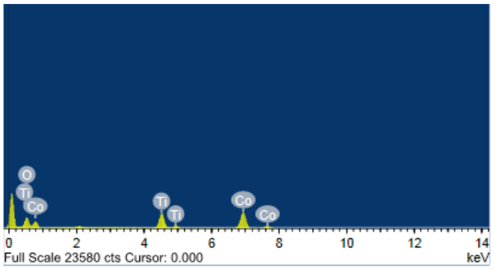


**Position 3**

| Elem... | Weight% | Atomic% |
|---|---|---|
| O K | 37.53 | 67.51 |
| Ti K | 17.57 | 10.56 |
| Co K | 44.90 | 21.93 |
| Totals | 100.00 | |

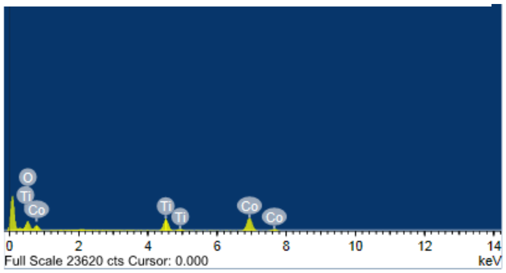


Figure S2. EDX spectra with the atomic percentage of CTO-Sp for three different positions of the sample surface.

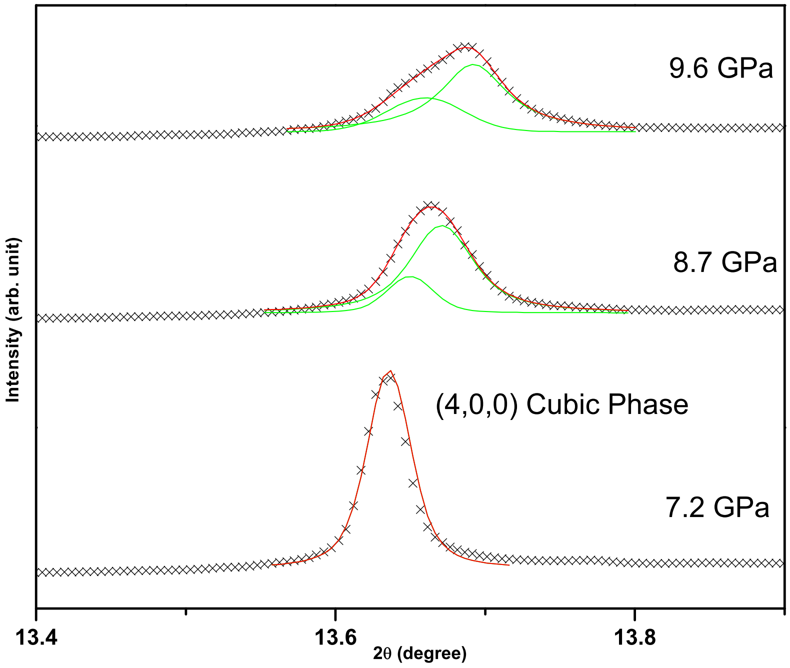


Figure S3. Splitting of (4,0,0) Brag peak in the cubic phase at and above 8.7 GPa.
